# Supplementary material for: Fast Fourier Intrinsic Network
Source: arXiv:2011.04612 source file (2020-11-09)
Supplement: Supplementary file 1 [file fig-iiw-supple.tex]

\begin{figure*}[htb]
  \centering
    \begin{tabular}{@{}c@{}c@{}c@{}c@{}c@{}c@{}c@{}c@{}c@{}}

        \vspace{-1mm}
        \\  
        \includegraphics[width=0.11\textwidth,height=0.07\textwidth]{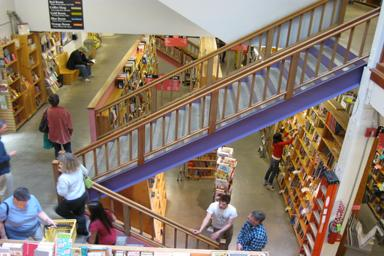} &
        \includegraphics[width=0.11\textwidth,height=0.07\textwidth]{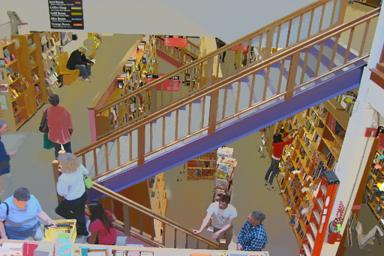} &
        \includegraphics[width=0.11\textwidth,height=0.07\textwidth]{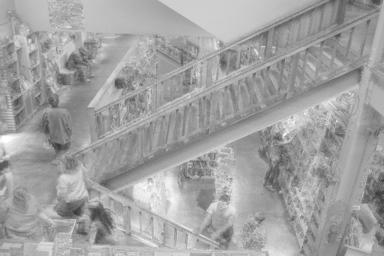} &
        \includegraphics[width=0.11\textwidth,height=0.07\textwidth]{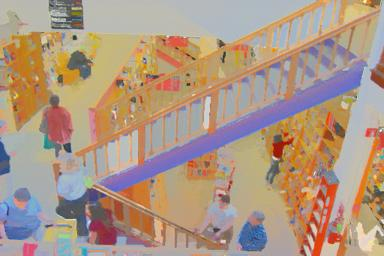} & 
		\includegraphics[width=0.11\textwidth,height=0.07\textwidth]{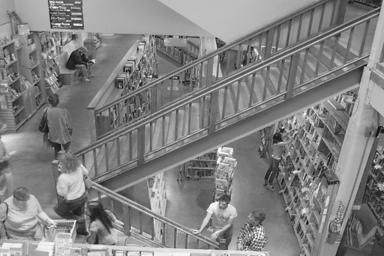} &         
        \includegraphics[width=0.11\textwidth,height=0.07\textwidth]{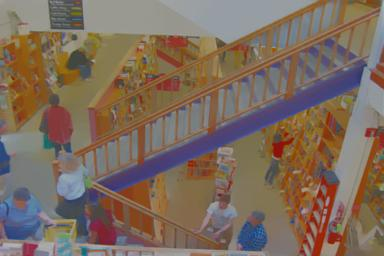}  & 
        \includegraphics[width=0.11\textwidth,height=0.07\textwidth]{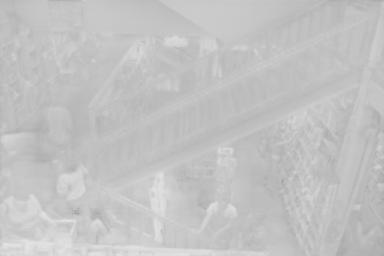} &
        \includegraphics[width=0.11\textwidth,height=0.07\textwidth]{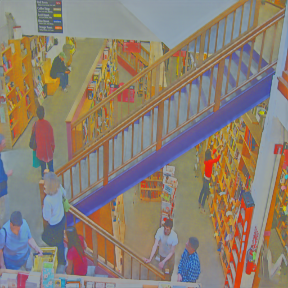}& 
        \includegraphics[width=0.11\textwidth,height=0.07\textwidth]{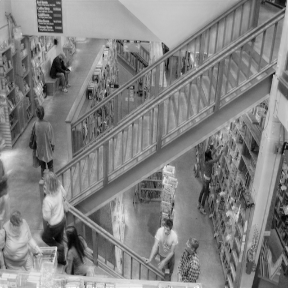}
  
          \vspace{-1mm}
        \\  
        %% 3rd row
        \includegraphics[width=0.11\textwidth,height=0.07\textwidth]{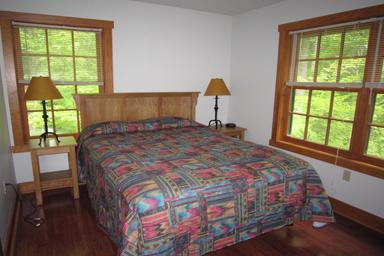} &
        \includegraphics[width=0.11\textwidth,height=0.07\textwidth]{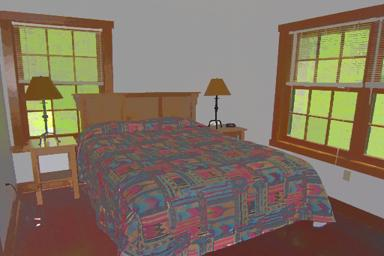} &
        \includegraphics[width=0.11\textwidth,height=0.07\textwidth]{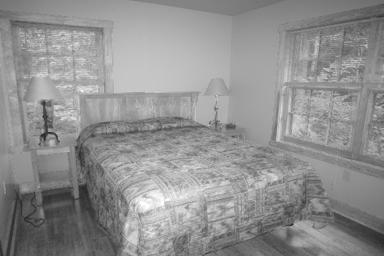} &
        \includegraphics[width=0.11\textwidth,height=0.07\textwidth]{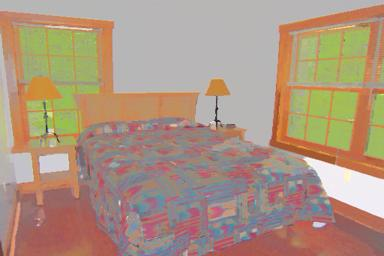} & 
		\includegraphics[width=0.11\textwidth,height=0.07\textwidth]{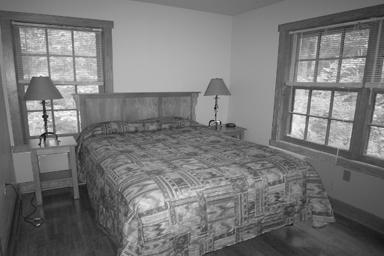} &         
        \includegraphics[width=0.11\textwidth,height=0.07\textwidth]{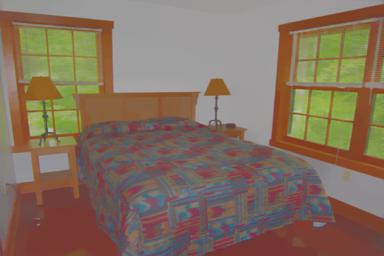}  & 
        \includegraphics[width=0.11\textwidth,height=0.07\textwidth]{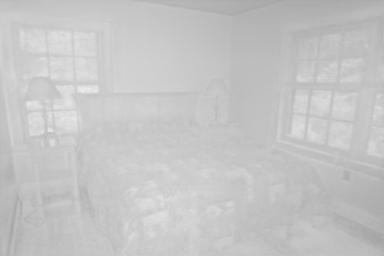} &
        \includegraphics[width=0.11\textwidth,height=0.07\textwidth]{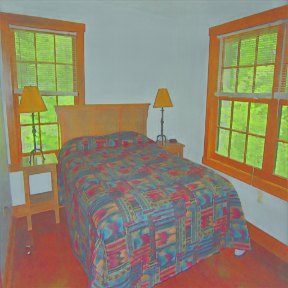}& 
                \includegraphics[width=0.11\textwidth,height=0.07\textwidth]{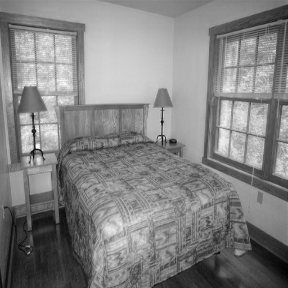}
                
%           \vspace{-1mm}
%         \\  
%         \includegraphics[width=0.11\textwidth,height=0.07\textwidth]{comp_iiw_supple/34735_img.jpg} &
%         \includegraphics[width=0.11\textwidth,height=0.07\textwidth]{comp_iiw_supple/34735_bell_A.jpg} &
%         \includegraphics[width=0.11\textwidth,height=0.07\textwidth]{comp_iiw_supple/34735_bell_S.jpg} &
%         \includegraphics[width=0.11\textwidth,height=0.07\textwidth]{comp_iiw_supple/34735_zhou_A.jpg} & 
% 		\includegraphics[width=0.11\textwidth,height=0.07\textwidth]{comp_iiw_supple/34735_zhou_S.jpg} &         
%         \includegraphics[width=0.11\textwidth,height=0.07\textwidth]{comp_iiw_supple/34735_cg_A.jpg}  & 
%         \includegraphics[width=0.11\textwidth,height=0.07\textwidth]{comp_iiw_supple/34735_cg_S.jpg} &
%         \includegraphics[width=0.11\textwidth,height=0.07\textwidth]{comp_iiw_supple/34735-albedo.png}& 
%         \includegraphics[width=0.11\textwidth,height=0.07\textwidth]{comp_iiw_supple/34735-shading.png}

                  \vspace{-1mm}
        \\  
        \includegraphics[width=0.11\textwidth,height=0.07\textwidth]{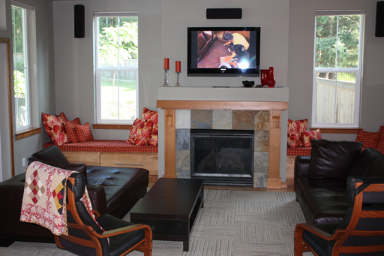} &
        \includegraphics[width=0.11\textwidth,height=0.07\textwidth]{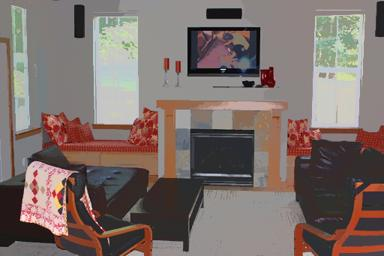} &
        \includegraphics[width=0.11\textwidth,height=0.07\textwidth]{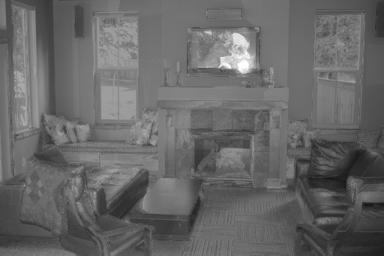} &
        \includegraphics[width=0.11\textwidth,height=0.07\textwidth]{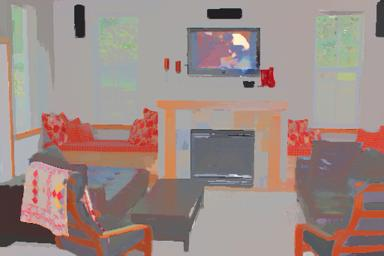} & 
		\includegraphics[width=0.11\textwidth,height=0.07\textwidth]{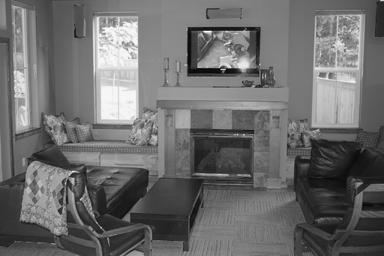} &         
        \includegraphics[width=0.11\textwidth,height=0.07\textwidth]{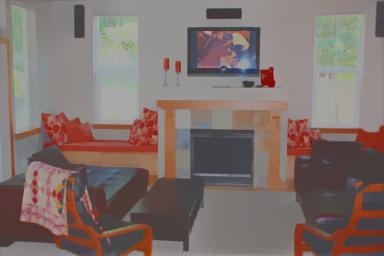}  & 
        \includegraphics[width=0.11\textwidth,height=0.07\textwidth]{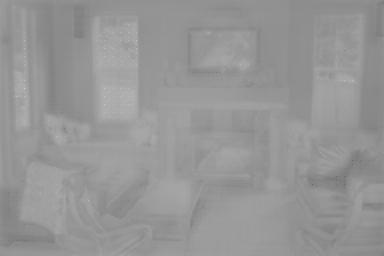} &
        \includegraphics[width=0.11\textwidth,height=0.07\textwidth]{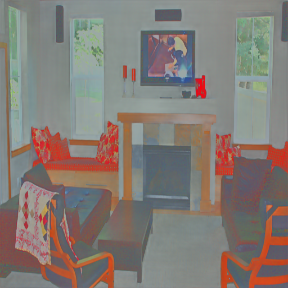}& 
        \includegraphics[width=0.11\textwidth,height=0.07\textwidth]{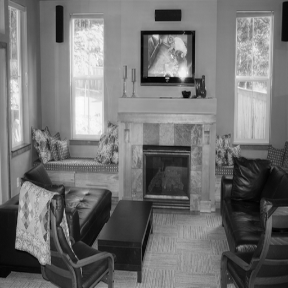}

                  \vspace{-1mm}
        \\  
        \includegraphics[width=0.11\textwidth,height=0.07\textwidth]{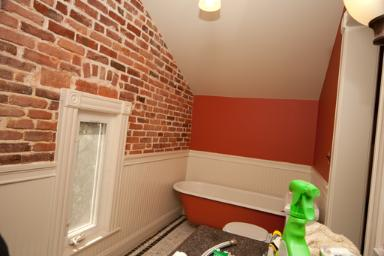} &
        \includegraphics[width=0.11\textwidth,height=0.07\textwidth]{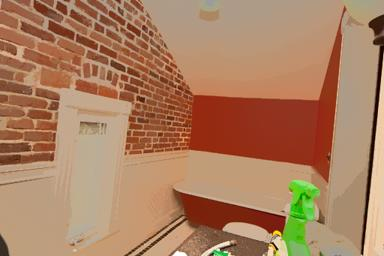} &
        \includegraphics[width=0.11\textwidth,height=0.07\textwidth]{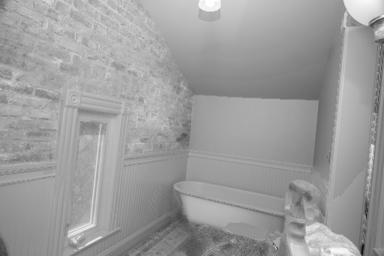} &
        \includegraphics[width=0.11\textwidth,height=0.07\textwidth]{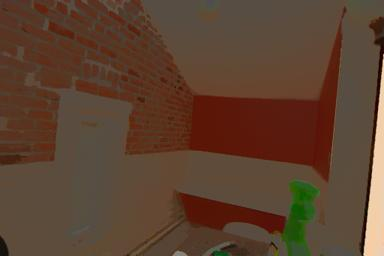} & 
		\includegraphics[width=0.11\textwidth,height=0.07\textwidth]{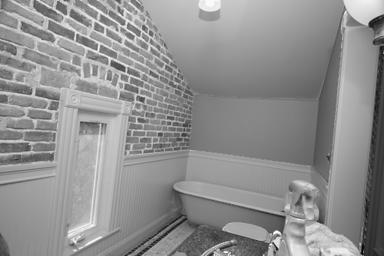} &         
        \includegraphics[width=0.11\textwidth,height=0.07\textwidth]{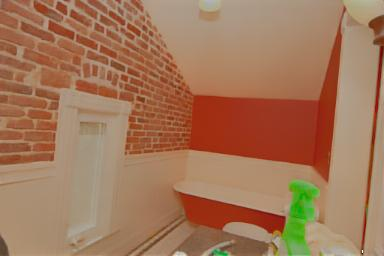}  & 
        \includegraphics[width=0.11\textwidth,height=0.07\textwidth]{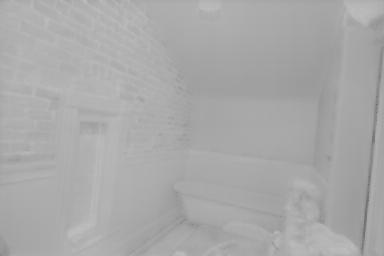} &
        \includegraphics[width=0.11\textwidth,height=0.07\textwidth]{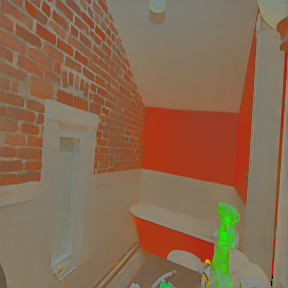}& 
        \includegraphics[width=0.11\textwidth,height=0.07\textwidth]{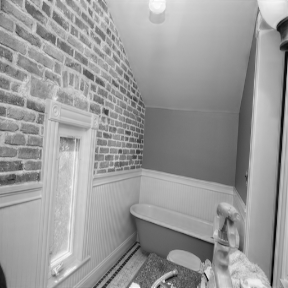}

%         \vspace{-1mm}
%         \\  
%         %% 3rd row
%         \includegraphics[width=0.11\textwidth,height=0.07\textwidth]{comp_iiw/img/118514.jpg} &
%         \includegraphics[width=0.11\textwidth,height=0.07\textwidth]{comp_iiw/bell/118514-r.jpg} &
%         \includegraphics[width=0.11\textwidth,height=0.07\textwidth]{comp_iiw/bell/118514-s.jpg} &
%         \includegraphics[width=0.11\textwidth,height=0.07\textwidth]{comp_iiw/zhou/118514-r.jpg} & 
% 		\includegraphics[width=0.11\textwidth,height=0.07\textwidth]{comp_iiw/zhou/118514-s.jpg} &         
%         \includegraphics[width=0.11\textwidth,height=0.07\textwidth]{comp_iiw/cg/118514-r.jpg}  & 
%         \includegraphics[width=0.11\textwidth,height=0.07\textwidth]{comp_iiw/cg/118514-s.jpg} &
%         \includegraphics[width=0.11\textwidth,height=0.07\textwidth]{comp_iiw/ffi/118514-albedo.png}& 
%         \includegraphics[width=0.11\textwidth,height=0.07\textwidth]{comp_iiw/ffi/118514-shading.png}

         \vspace{-1mm}
        \\                       
        {\scriptsize Image} & {\scriptsize Bell~\cite{bell2014intrinsic} ($A$)}  & {\scriptsize Bell~\cite{bell2014intrinsic}($S$)} & {\scriptsize Zhou~\cite{zhou2015learning} ($A$)}  & {\scriptsize Zhou \cite{zhou2015learning} ($S$)}  & {\scriptsize CGI \cite{cgintrinsic} ($A$)} & {\scriptsize CGI \cite{cgintrinsic} ($S$)}   &  {\scriptsize FFI-Net ($A$)} & {\scriptsize FFI-Net ($S$)}
    \end{tabular}  
  \caption{ Qualitative comparisons of (A)lebdo and (S)hading on IIW.
    % Our predictions show significant improvements compared to
    % state-of-the-art algorithms (bell~\etal ~\cite{bell2014intrinsic}
    % and zhou~\etal~\cite{zhou2015learning}). 
    % In particular, our
    % predicted shading channels include significantly less surface
    % texture in several challenging
    % settings.
    } \label{fig:iiw} 
\end{figure*}
