# Supplementary material for: Fast Fourier Intrinsic Network
Source: arXiv:2011.04612 source file (2020-11-09)
Supplement: Supplementary file 2 [file fig-mit-supple.tex]

\begin{figure}[htp]
\begin{center}
\resizebox{1.0\linewidth}{!}{
\begin{tabular}{c c ccccc}
\vspace{-0.5mm}
\!\!\includegraphics[width=1.4cm]{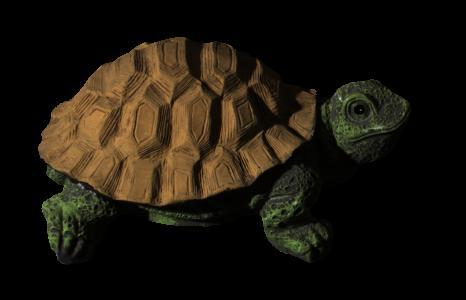}
& \raisebox{3mm}{\rotatebox{0}{(A)}}
&\includegraphics[width=1.4cm]{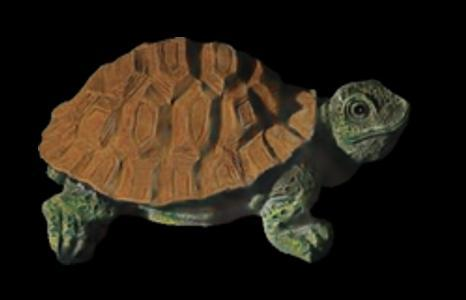}
&\includegraphics[width=1.4cm]{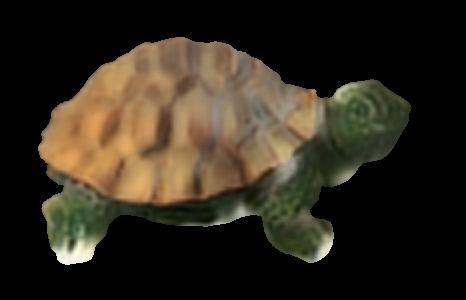}
&\includegraphics[width=1.4cm]{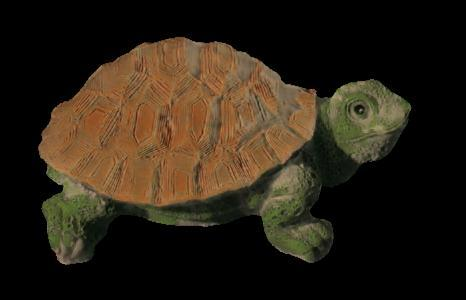}
&\includegraphics[width=1.4cm]{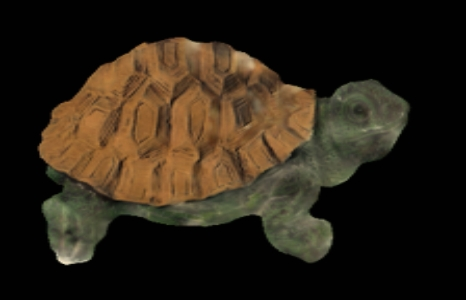}
&\includegraphics[width=1.4cm]{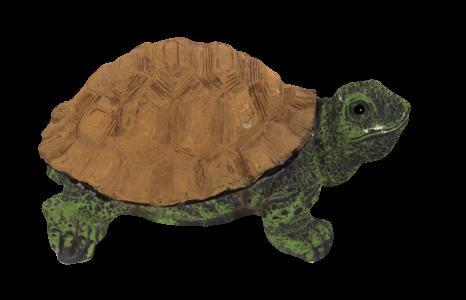}\cr
& \raisebox{3mm}{\rotatebox{0}{(S)}}
&\includegraphics[width=1.4cm]{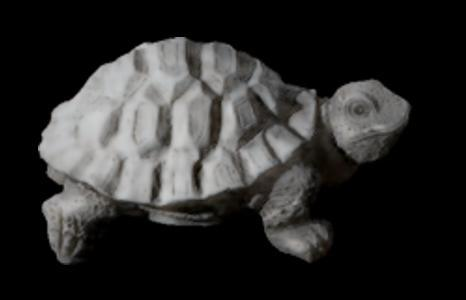}
&\includegraphics[width=1.4cm]{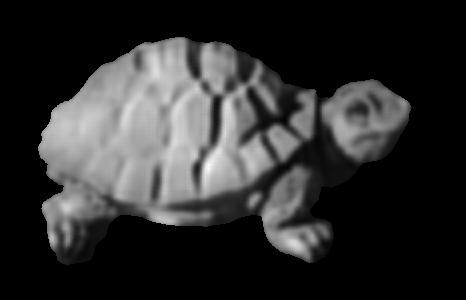}
&\includegraphics[width=1.4cm]{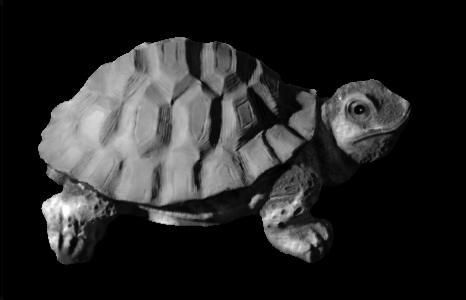}
&\includegraphics[width=1.4cm]{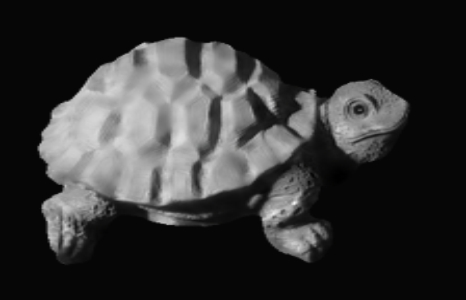}
&\includegraphics[width=1.4cm]{comp_MIT/turtle_predict_shading.jpg}\\

\vspace{-0.5mm}

\!\!\includegraphics[width=1.4cm]{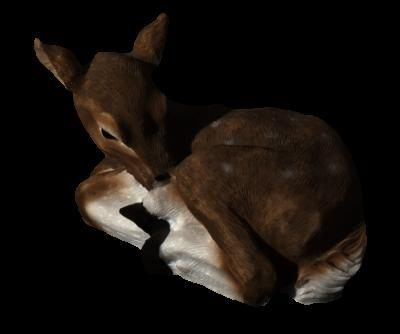}
& \raisebox{3mm}{\rotatebox{0}{(A)}}
&\includegraphics[width=1.4cm]{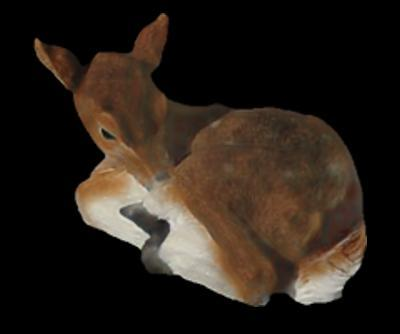}
&\includegraphics[width=1.4cm]{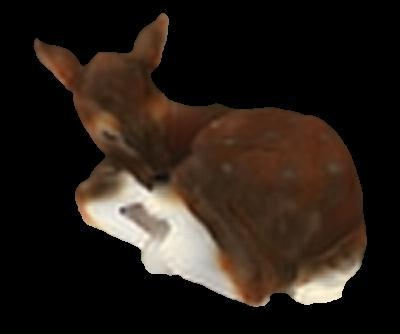}
&\includegraphics[width=1.4cm]{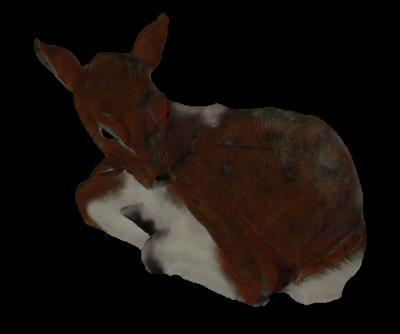}
&\includegraphics[width=1.4cm]{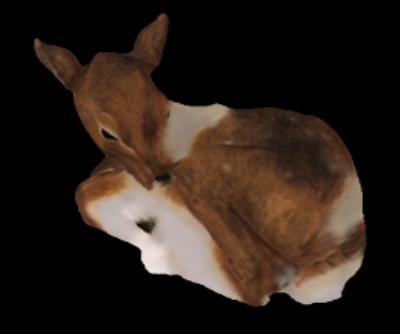}
&\includegraphics[width=1.4cm]{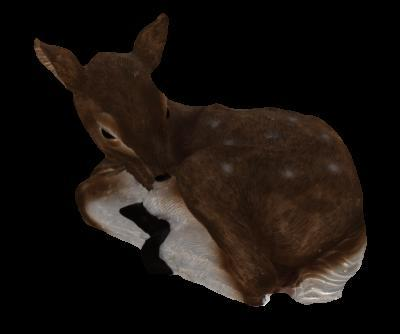}
\\
& \raisebox{3mm}{\rotatebox{0}{(S)}}
&\includegraphics[width=1.4cm]{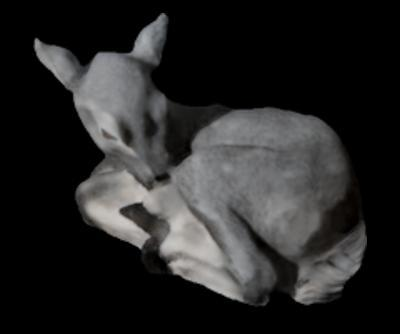}
&\includegraphics[width=1.4cm]{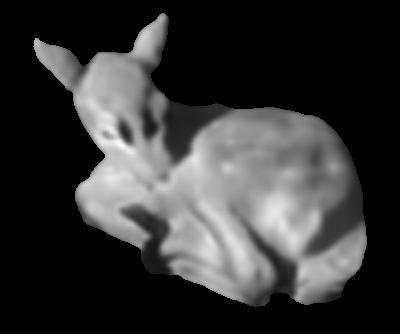}
&\includegraphics[width=1.4cm,,height=1.215cm]{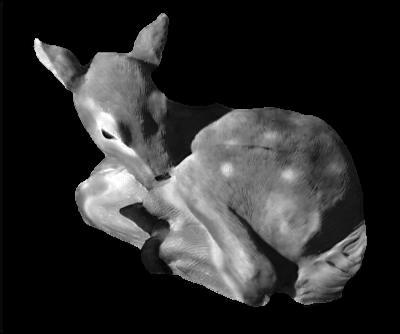}
&\includegraphics[width=1.4cm, height=1.215cm]{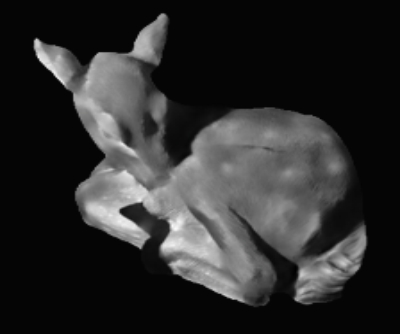}
&\includegraphics[width=1.4cm]{comp_MIT/deer_predict_shading.jpg}\\

%\vspace{-0.75mm}
%
%\includegraphics[width=1.4cm]{pear-1-input.jpg}
%
%&\includegraphics[width=1.4cm]{pear-1-predict-albedo-Shijian.jpg}
%&\includegraphics[width=1.4cm]{pear-1-predict-albedo-DI.jpg}
%&\includegraphics[width=1.4cm]{pear-1-predict-albedo.jpg}
%&\includegraphics[width=1.4cm]{pear-1-labelA.jpg}
%
%&\includegraphics[width=1.4cm]{pear-1-predict-shading-Shijian.jpg}
%&\includegraphics[width=1.4cm]{pear-1-predict-shading-DI.jpg}
%&\includegraphics[width=1.4cm]{pear-1-predict-shading.jpg}
%&\includegraphics[width=1.4cm]{pear-1-labelS.jpg}\\

%\vspace{-0.75mm}
%
%\includegraphics[width=1.4cm]{turtle-1-input.jpg}
%&\includegraphics[width=1.4cm]{turtle-1-predict-albedo-Shijian.jpg}
%&\includegraphics[width=1.4cm]{turtle-1-predict-albedo-DI.jpg}
%&\includegraphics[width=1.4cm]{turtle-1-predict-albedo.jpg}
%&\includegraphics[width=1.4cm]{turtle-1-labelA.jpg}
%&\includegraphics[width=1.4cm]{turtle-1-predict-shading-Shijian.jpg}
%&\includegraphics[width=1.4cm]{turtle-1-predict-shading-DI.jpg}
%&\includegraphics[width=1.4cm]{turtle-1-predict-shading.jpg}
%&\includegraphics[width=1.4cm]{turtle-1-labelS.jpg}\\

\vspace{-0.5mm}

\small{Input} & & \small{Shi \emph{et al.} \cite{shi2017learning}} & \small{DI \cite{narihira2015direct}} & \small{Fan \textit{et al.} \cite{fan2018revisiting}} & \small{FFI-Net} & \small{Ground Truth}\\

% \vspace{-0.6mm}

% &\multicolumn{4}{ c }{\small{Albedo}} & \multicolumn{4}{ c }{\small{Shading}}\\
\end{tabular}}

\end{center}
\vspace{-2mm}
\caption{Sample  (A)lbedo and (S)hading on MIT Intrinsic. 
%Only trained on MIT itself, our method can produce visually-pleasing output, similiar to Fan \textit{et al.} \cite{fan2018revisiting}
}
\label{figure:mit-supple}
\vspace{-0mm}
\end{figure}
