# Supplementary material for: Fast Fourier Intrinsic Network
Source: arXiv:2011.04612 source file (2020-11-09)
Supplement: Supplementary file 3 [file fig-mpi-imagesplit-supple.tex]

\begin{figure}[t]
\begin{center}

\begin{tabular}{ccc}

\vspace{-0.75mm}
\raisebox{.9\height}{\rotatebox{90}{\scriptsize{{Input}}}}
&\multicolumn{2}{c}{\includegraphics[width=3.6cm]{comp-mpi-imagesplit/2-input.jpg}}
\\
& (A) & (S) \\
% \vspace{-0.75mm}
% \raisebox{0.5\height}{\rotatebox{90}{\scriptsize{{Lee~\cite{lee2012estimation}}}}}
% &{{\includegraphics[width=3.6cm]{comp-mpi-imagesplit/2-predict-albedo-lee.jpg}}}
% &{{\includegraphics[width=3.6cm]{comp-mpi-imagesplit/2-predict-shading-lee.jpg}}}
% \\

\vspace{-0.75mm}
\raisebox{0.5\height}{\rotatebox{90}{\scriptsize{{Barron~\cite{barron2015shape}}}}}
&{{\includegraphics[width=3.6cm]{comp-mpi-imagesplit/2-predict-albedo-barron.jpg}}}
&{{\includegraphics[width=3.6cm]{comp-mpi-imagesplit/2-predict-shading-barron.jpg}}}
\\

\vspace{-0.75mm}
\raisebox{0.5\height}{\rotatebox{90}{\scriptsize{{Chen~\cite{chen2013simple}}}}}
&{{\includegraphics[width=3.6cm]{comp-mpi-imagesplit/2-predict-albedo-chen.jpg}}}
&{{\includegraphics[width=3.6cm]{comp-mpi-imagesplit/2-predict-shading-chen.jpg}}}
\\

\vspace{-0.75mm}
\raisebox{1\height}{\rotatebox{90}{\scriptsize{{DI~\cite{narihira2015direct}}}}}
&{{\includegraphics[width=3.6cm]{comp-mpi-imagesplit/2-predict-albedo-di.jpg}}}
&{{\includegraphics[width=3.6cm]{comp-mpi-imagesplit/2-predict-shading-di.jpg}}}
\\

\vspace{-0.75mm}
\raisebox{1\height}{\rotatebox{90}{\scriptsize{{Fan \cite{fan2018revisiting}}}}}
&{{\includegraphics[width=3.6cm]{comp-mpi-imagesplit/2-predict-albedo-fan.jpg}}}
&{{\includegraphics[width=3.6cm]{comp-mpi-imagesplit/2-predict-shading-fan.jpg}}}
\\

\vspace{-0.75mm}
\raisebox{1\height}{\rotatebox{90}{\scriptsize{{Lap\cite{cheng2018intrinsic}}}}}
&{{\includegraphics[width=3.6cm]{comp-mpi-imagesplit/2-predict-albedo-lap.jpg}}}
&{{\includegraphics[width=3.6cm]{comp-mpi-imagesplit/2-predict-shading-lap.jpg}}}
\\

\vspace{-0.75mm}
\raisebox{1\height}{\rotatebox{90}{\scriptsize{{~~~~FFI}}}}
&{{\includegraphics[width=3.6cm]{comp-mpi-imagesplit/2-predict-albedo-fft.png}}}
&{{\includegraphics[width=3.6cm]{comp-mpi-imagesplit/2-predict-shading-fft.png}}}
\\

\vspace{-0.75mm}
{\rotatebox{90}{\scriptsize{{Ground Truth}}}}
&{{\includegraphics[width=3.6cm]{comp-mpi-imagesplit/2-label-albedo-mark.jpg}}}
&{{\includegraphics[width=3.6cm]{comp-mpi-imagesplit/2-label-shading-mark.jpg}}}
\\
\vspace{-5mm}

\end{tabular}

\end{center}
\vspace{-2.5mm}
\caption{More Examples of (A)lbedo and (S)hading predictions on MPI-Sintel (image split). %FFI-Net performs well in difficult parts, \eg hair bunchesa and  cast shadows.
}
\label{figure:mpi_imagesplit_supple}
\vspace{-3mm}
\end{figure}

%Compared to state-of-the-art method MSCR \cite{DI2015}, we show much sharper effects and better performance.
