# Supplementary material for: Fast Fourier Intrinsic Network
Source: arXiv:2011.04612 source file (2020-11-09)
Supplement: Supplementary file 4 [file fig-mpi-scensplit-supple.tex]

\setlength{\tabcolsep}{1pt}

\begin{figure}
\begin{center}
\vspace{-3mm}
\begin{tabular}{ccc}

%\vspace{-0.75mm}
%\raisebox{.9\height}{\rotatebox{90}{\scriptsize{{Input}}}}&\multicolumn{2}{c}{\includegraphics[width=3.6cm]{comp-mpi-scenesplit/sleeping_2_frame_0014-input.jpg}}\\& (A) & (S) \\
%\vspace{-0.75mm}
%\raisebox{1\height}{\rotatebox{90}{\scriptsize{{DI~\cite{narihira2015direct}}}}}&{{\includegraphics[width=3.6cm]{comp-mpi-scenesplit/sleeping_2_frame_0014-predict-albedo-MSCR.jpg}}}&{{\includegraphics[width=3.6cm]{comp-mpi-scenesplit/sleeping_2_frame_0014-predict-shading-MSCR.jpg}}}\\

%\vspace{-0.75mm} \raisebox{1\height}{\rotatebox{90}{\scriptsize{{Fan \cite{fan2018revisiting}}}}}&{{\includegraphics[width=3.6cm]{comp-mpi-scenesplit/sleeping_2_frame_0014-predict-albedo-fan.jpg}}}&{{\includegraphics[width=3.6cm]{comp-mpi-scenesplit/sleeping_2_frame_0014-predict-shading-fan.jpg}}}\\

%\vspace{-0.75mm}
%\raisebox{1\height}{\rotatebox{90}{\scriptsize{{~~~~FFI}}}}&{{\includegraphics[width=3.6cm]{comp-mpi-scenesplit/sleeping_2_frame_0014-predict-albedo.jpg}}}&{{\includegraphics[width=3.6cm]{comp-mpi-scenesplit/sleeping_2_frame_0014-predict-shading.jpg}}}\\

%\vspace{-0.75mm}
%{\rotatebox{90}{\scriptsize{{Ground Truth}}}}&{{\includegraphics[width=3.6cm]{comp-mpi-scenesplit/sleeping_2_frame_0014-label-albedo.jpg}}}&{{\includegraphics[width=3.6cm]{comp-mpi-scenesplit/sleeping_2_frame_0014-label-shading.jpg}}}\vspace{5mm}\\

\raisebox{.9\height}{\rotatebox{90}{\scriptsize{{Input}}}}
&\multicolumn{2}{c}{\includegraphics[width=3.6cm]{comp-mpi-scenesplit/market_6_frame_0012-input.jpg}}
\\
& (A) & (S) \\
\vspace{-0.75mm}
\raisebox{1\height}{\rotatebox{90}{\scriptsize{{DI~\cite{narihira2015direct}}}}}
&{{\includegraphics[width=3.6cm]{comp-mpi-scenesplit/market_6_frame_0012-predict-albedo-MSCR.jpg}}}
&{{\includegraphics[width=3.6cm]{comp-mpi-scenesplit/market_6_frame_0012-predict-shading-MSCR.jpg}}}
\\

\vspace{-0.75mm}
\raisebox{1\height}{\rotatebox{90}{\scriptsize{{Fan \cite{fan2018revisiting}}}}}
&{{\includegraphics[width=3.6cm]{comp-mpi-scenesplit/market_6_frame_0012-predict-albedo-fan.jpg}}}
&{{\includegraphics[width=3.6cm]{comp-mpi-scenesplit/market_6_frame_0012-predict-shading-fan.jpg}}}
\\

\vspace{-0.75mm}
\raisebox{1\height}{\rotatebox{90}{\scriptsize{{~~~~FFI}}}}
&{{\includegraphics[width=3.6cm]{comp-mpi-scenesplit/market_6_frame_0012-predict-albedo.jpg}}}
&{{\includegraphics[width=3.6cm]{comp-mpi-scenesplit/market_6_frame_0012-predict-shading.jpg}}}
\\

\vspace{-0.75mm}
{\rotatebox{90}{\scriptsize{{Ground Truth}}}}
&{{\includegraphics[width=3.6cm]{comp-mpi-scenesplit/market_6_frame_0012-label-albedo-mark.jpg}}}
&{{\includegraphics[width=3.6cm]{comp-mpi-scenesplit/market_6_frame_0012-label-shading-mark.jpg}}}
\\

\vspace{-5mm}

\end{tabular}

\end{center}
\vspace{-2.5mm}
\caption{Examples on the MPI-Sintel dataset (scene split). }
\label{figure:mpi_scenesplit_supple}
%\vspace{-3mm}
\end{figure}

%Compared to state-of-the-art method MSCR \cite{DI2015}, we show much sharper effects and better performance.
