# Supplementary material for: Fast Fourier Intrinsic Network
Source: arXiv:2011.04612 source file (2020-11-09)
Supplement: Supplementary file 5 [file supplement.tex]

\emph{This supplementary material provides %1) the pseudo code for the conjugate symmetry constraint in FFI-Net, which accepts arbitrary input size; 2) 
1) the training\&testing splits for MPI-Sintel and MIT Intrinsic; 2) more examples for visualization and comparison.  }

\section{Training\&Testing Splits}
We use the same training\&testing split files with \cite{narihira2015direct} and \cite{barron2015shape} for MIP-Sintel and MIT Intrinsic, respectively. 
We think it would be good to publish these files such that any following-up works can use them and make a fair comparison with us or any previous relevant works. We report the scene-split for MPI-Sintel and object-split for MIT Intrinsic dataset below.

\vspace{5mm}
\noindent \textbf{MPI-Sintel}: \\
\emph{training}: alley\_1, bamboo\_1, bandage\_1,cave\_2,market\_2, market\_6, shaman\_2, sleeping\_1, temple\_2 \\
\emph{testing}: alley\_2, bamboo\_2, bandage\_2, cave\_4, market\_5, mountain\_1, shaman\_3, sleeping\_2, temple\_3

\noindent \textbf{MIT Intrinsic}: \\
\emph{training}: apple,box, cup1, dinosaur, frog1, panther, paper1, phone, squirrel, teabag2 \\
\emph{testing}: cup2, deer, frog2, paper2, pear, potato, raccoon, sun, teabag1, turtle

\setlength{\tabcolsep}{1pt}

\begin{figure}
\begin{center}
\vspace{-3mm}
\begin{tabular}{ccc}

%\vspace{-0.75mm}
%\raisebox{.9\height}{\rotatebox{90}{\scriptsize{{Input}}}}&\multicolumn{2}{c}{\includegraphics[width=3.6cm]{comp-mpi-scenesplit/sleeping_2_frame_0014-input.jpg}}\\& (A) & (S) \\
%\vspace{-0.75mm}
%\raisebox{1\height}{\rotatebox{90}{\scriptsize{{DI~\cite{narihira2015direct}}}}}&{{\includegraphics[width=3.6cm]{comp-mpi-scenesplit/sleeping_2_frame_0014-predict-albedo-MSCR.jpg}}}&{{\includegraphics[width=3.6cm]{comp-mpi-scenesplit/sleeping_2_frame_0014-predict-shading-MSCR.jpg}}}\\

%\vspace{-0.75mm} \raisebox{1\height}{\rotatebox{90}{\scriptsize{{Fan \cite{fan2018revisiting}}}}}&{{\includegraphics[width=3.6cm]{comp-mpi-scenesplit/sleeping_2_frame_0014-predict-albedo-fan.jpg}}}&{{\includegraphics[width=3.6cm]{comp-mpi-scenesplit/sleeping_2_frame_0014-predict-shading-fan.jpg}}}\\

%\vspace{-0.75mm}
%\raisebox{1\height}{\rotatebox{90}{\scriptsize{{~~~~FFI}}}}&{{\includegraphics[width=3.6cm]{comp-mpi-scenesplit/sleeping_2_frame_0014-predict-albedo.jpg}}}&{{\includegraphics[width=3.6cm]{comp-mpi-scenesplit/sleeping_2_frame_0014-predict-shading.jpg}}}\\

%\vspace{-0.75mm}
%{\rotatebox{90}{\scriptsize{{Ground Truth}}}}&{{\includegraphics[width=3.6cm]{comp-mpi-scenesplit/sleeping_2_frame_0014-label-albedo.jpg}}}&{{\includegraphics[width=3.6cm]{comp-mpi-scenesplit/sleeping_2_frame_0014-label-shading.jpg}}}\vspace{5mm}\\

\raisebox{.9\height}{\rotatebox{90}{\scriptsize{{Input}}}}
&\multicolumn{2}{c}{\includegraphics[width=3.6cm]{comp-mpi-scenesplit/market_6_frame_0012-input.jpg}}
\\
& (A) & (S) \\
\vspace{-0.75mm}
\raisebox{1\height}{\rotatebox{90}{\scriptsize{{DI~\cite{narihira2015direct}}}}}
&{{\includegraphics[width=3.6cm]{comp-mpi-scenesplit/market_6_frame_0012-predict-albedo-MSCR.jpg}}}
&{{\includegraphics[width=3.6cm]{comp-mpi-scenesplit/market_6_frame_0012-predict-shading-MSCR.jpg}}}
\\

\vspace{-0.75mm}
\raisebox{1\height}{\rotatebox{90}{\scriptsize{{Fan \cite{fan2018revisiting}}}}}
&{{\includegraphics[width=3.6cm]{comp-mpi-scenesplit/market_6_frame_0012-predict-albedo-fan.jpg}}}
&{{\includegraphics[width=3.6cm]{comp-mpi-scenesplit/market_6_frame_0012-predict-shading-fan.jpg}}}
\\

\vspace{-0.75mm}
\raisebox{1\height}{\rotatebox{90}{\scriptsize{{~~~~FFI}}}}
&{{\includegraphics[width=3.6cm]{comp-mpi-scenesplit/market_6_frame_0012-predict-albedo.jpg}}}
&{{\includegraphics[width=3.6cm]{comp-mpi-scenesplit/market_6_frame_0012-predict-shading.jpg}}}
\\

\vspace{-0.75mm}
{\rotatebox{90}{\scriptsize{{Ground Truth}}}}
&{{\includegraphics[width=3.6cm]{comp-mpi-scenesplit/market_6_frame_0012-label-albedo-mark.jpg}}}
&{{\includegraphics[width=3.6cm]{comp-mpi-scenesplit/market_6_frame_0012-label-shading-mark.jpg}}}
\\

\vspace{-5mm}

\end{tabular}

\end{center}
\vspace{-2.5mm}
\caption{Examples on the MPI-Sintel dataset (scene split). }
\label{figure:mpi_scenesplit_supple}
%\vspace{-3mm}
\end{figure}

%Compared to state-of-the-art method MSCR \cite{DI2015}, we show much sharper effects and better performance.

\begin{figure*}[htb]
  \centering
    \begin{tabular}{@{}c@{}c@{}c@{}c@{}c@{}c@{}c@{}c@{}c@{}}

        \vspace{-1mm}
        \\  
        \includegraphics[width=0.11\textwidth,height=0.07\textwidth]{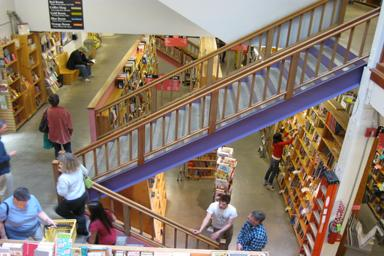} &
        \includegraphics[width=0.11\textwidth,height=0.07\textwidth]{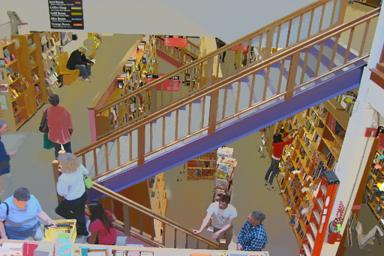} &
        \includegraphics[width=0.11\textwidth,height=0.07\textwidth]{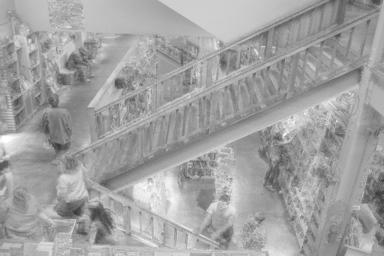} &
        \includegraphics[width=0.11\textwidth,height=0.07\textwidth]{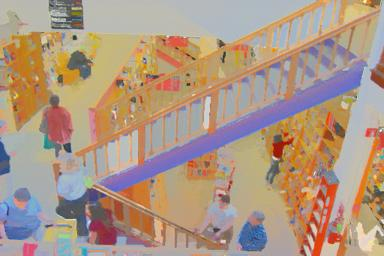} & 
		\includegraphics[width=0.11\textwidth,height=0.07\textwidth]{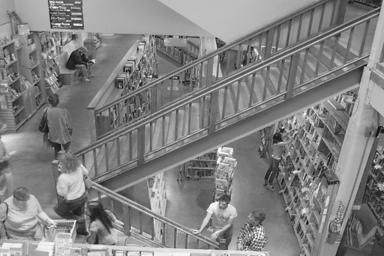} &         
        \includegraphics[width=0.11\textwidth,height=0.07\textwidth]{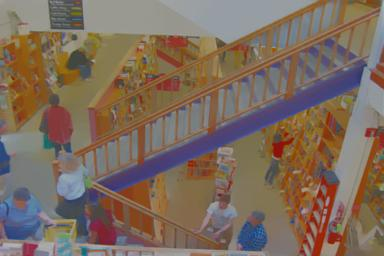}  & 
        \includegraphics[width=0.11\textwidth,height=0.07\textwidth]{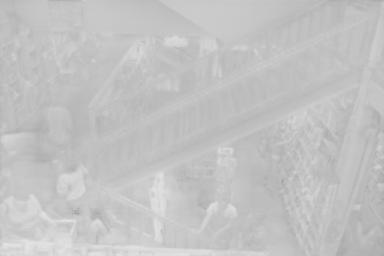} &
        \includegraphics[width=0.11\textwidth,height=0.07\textwidth]{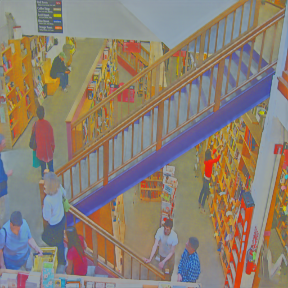}& 
        \includegraphics[width=0.11\textwidth,height=0.07\textwidth]{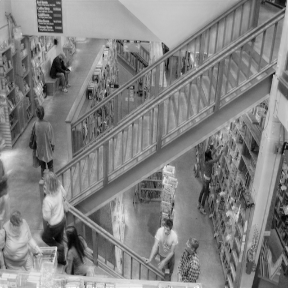}
  
          \vspace{-1mm}
        \\  
        %% 3rd row
        \includegraphics[width=0.11\textwidth,height=0.07\textwidth]{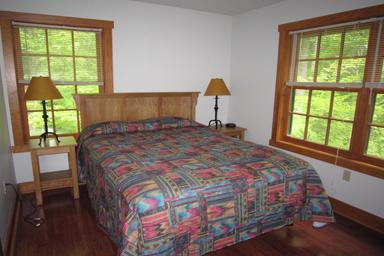} &
        \includegraphics[width=0.11\textwidth,height=0.07\textwidth]{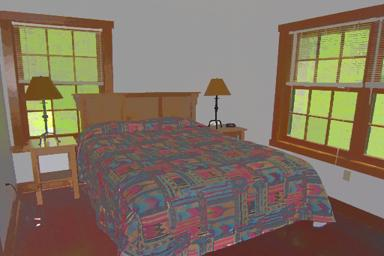} &
        \includegraphics[width=0.11\textwidth,height=0.07\textwidth]{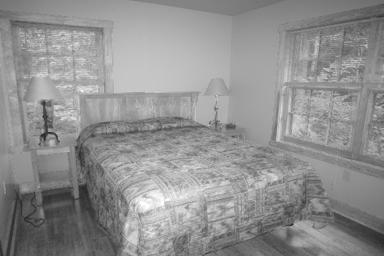} &
        \includegraphics[width=0.11\textwidth,height=0.07\textwidth]{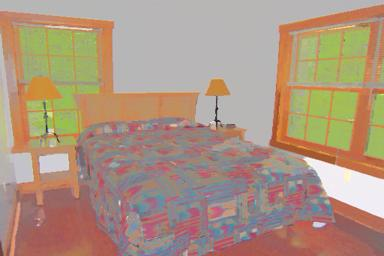} & 
		\includegraphics[width=0.11\textwidth,height=0.07\textwidth]{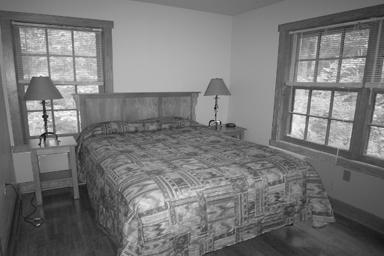} &         
        \includegraphics[width=0.11\textwidth,height=0.07\textwidth]{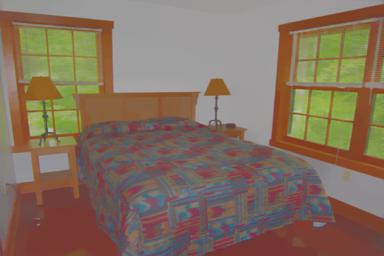}  & 
        \includegraphics[width=0.11\textwidth,height=0.07\textwidth]{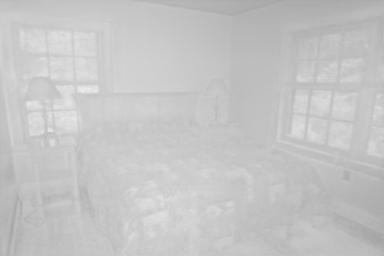} &
        \includegraphics[width=0.11\textwidth,height=0.07\textwidth]{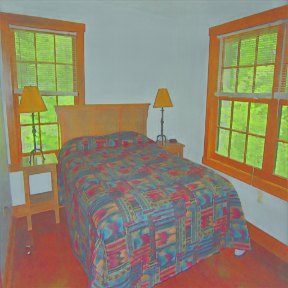}& 
                \includegraphics[width=0.11\textwidth,height=0.07\textwidth]{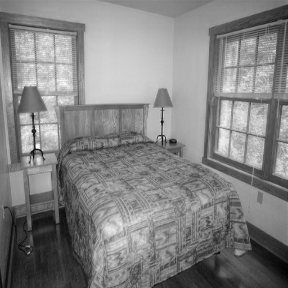}
                
%           \vspace{-1mm}
%         \\  
%         \includegraphics[width=0.11\textwidth,height=0.07\textwidth]{comp_iiw_supple/34735_img.jpg} &
%         \includegraphics[width=0.11\textwidth,height=0.07\textwidth]{comp_iiw_supple/34735_bell_A.jpg} &
%         \includegraphics[width=0.11\textwidth,height=0.07\textwidth]{comp_iiw_supple/34735_bell_S.jpg} &
%         \includegraphics[width=0.11\textwidth,height=0.07\textwidth]{comp_iiw_supple/34735_zhou_A.jpg} & 
% 		\includegraphics[width=0.11\textwidth,height=0.07\textwidth]{comp_iiw_supple/34735_zhou_S.jpg} &         
%         \includegraphics[width=0.11\textwidth,height=0.07\textwidth]{comp_iiw_supple/34735_cg_A.jpg}  & 
%         \includegraphics[width=0.11\textwidth,height=0.07\textwidth]{comp_iiw_supple/34735_cg_S.jpg} &
%         \includegraphics[width=0.11\textwidth,height=0.07\textwidth]{comp_iiw_supple/34735-albedo.png}& 
%         \includegraphics[width=0.11\textwidth,height=0.07\textwidth]{comp_iiw_supple/34735-shading.png}

                  \vspace{-1mm}
        \\  
        \includegraphics[width=0.11\textwidth,height=0.07\textwidth]{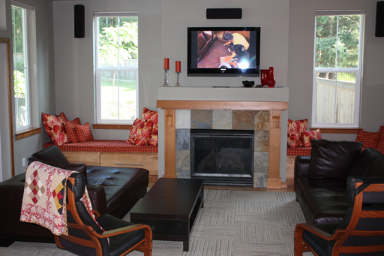} &
        \includegraphics[width=0.11\textwidth,height=0.07\textwidth]{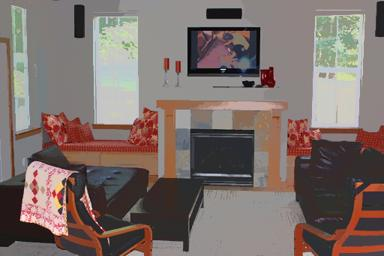} &
        \includegraphics[width=0.11\textwidth,height=0.07\textwidth]{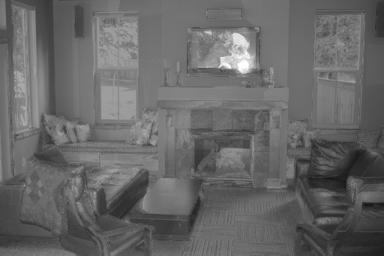} &
        \includegraphics[width=0.11\textwidth,height=0.07\textwidth]{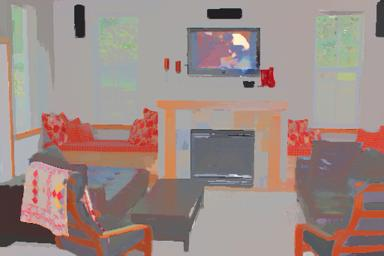} & 
		\includegraphics[width=0.11\textwidth,height=0.07\textwidth]{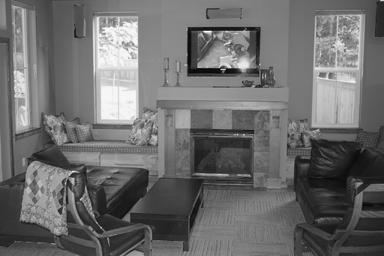} &         
        \includegraphics[width=0.11\textwidth,height=0.07\textwidth]{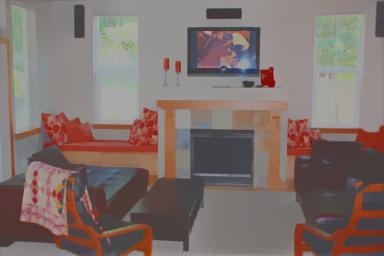}  & 
        \includegraphics[width=0.11\textwidth,height=0.07\textwidth]{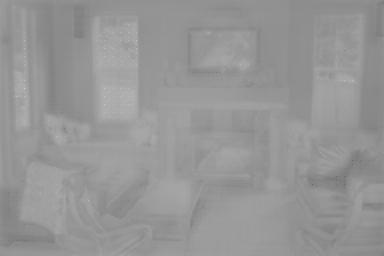} &
        \includegraphics[width=0.11\textwidth,height=0.07\textwidth]{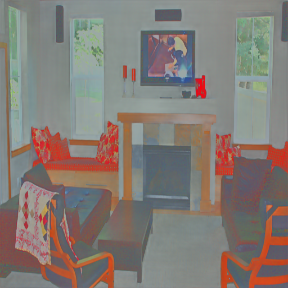}& 
        \includegraphics[width=0.11\textwidth,height=0.07\textwidth]{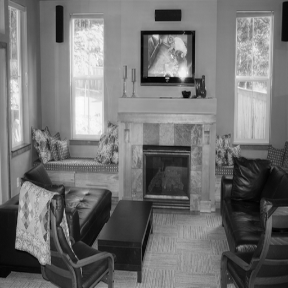}

                  \vspace{-1mm}
        \\  
        \includegraphics[width=0.11\textwidth,height=0.07\textwidth]{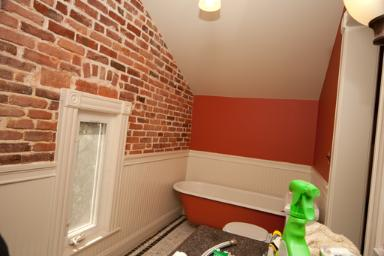} &
        \includegraphics[width=0.11\textwidth,height=0.07\textwidth]{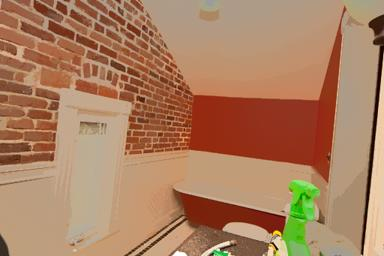} &
        \includegraphics[width=0.11\textwidth,height=0.07\textwidth]{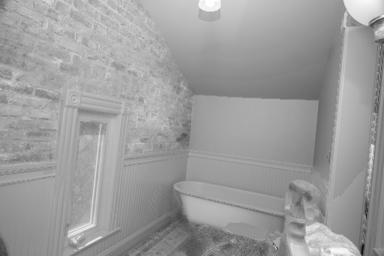} &
        \includegraphics[width=0.11\textwidth,height=0.07\textwidth]{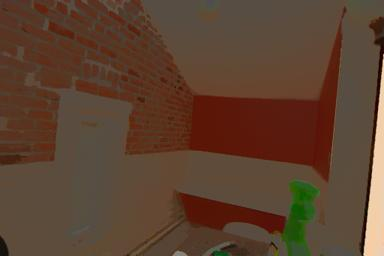} & 
		\includegraphics[width=0.11\textwidth,height=0.07\textwidth]{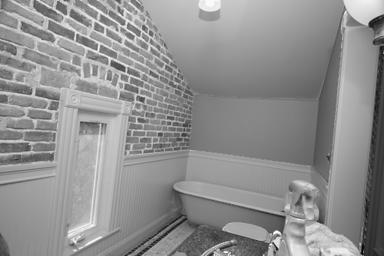} &         
        \includegraphics[width=0.11\textwidth,height=0.07\textwidth]{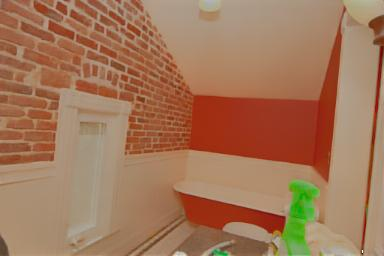}  & 
        \includegraphics[width=0.11\textwidth,height=0.07\textwidth]{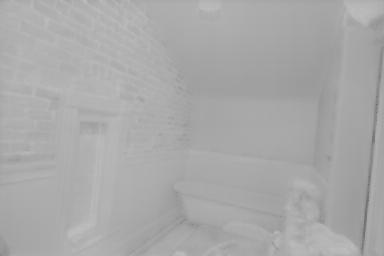} &
        \includegraphics[width=0.11\textwidth,height=0.07\textwidth]{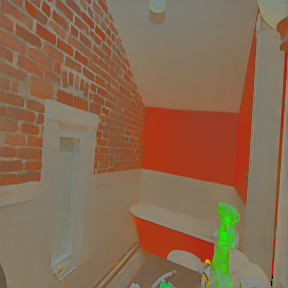}& 
        \includegraphics[width=0.11\textwidth,height=0.07\textwidth]{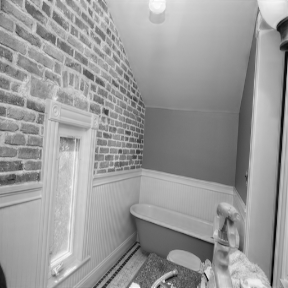}

%         \vspace{-1mm}
%         \\  
%         %% 3rd row
%         \includegraphics[width=0.11\textwidth,height=0.07\textwidth]{comp_iiw/img/118514.jpg} &
%         \includegraphics[width=0.11\textwidth,height=0.07\textwidth]{comp_iiw/bell/118514-r.jpg} &
%         \includegraphics[width=0.11\textwidth,height=0.07\textwidth]{comp_iiw/bell/118514-s.jpg} &
%         \includegraphics[width=0.11\textwidth,height=0.07\textwidth]{comp_iiw/zhou/118514-r.jpg} & 
% 		\includegraphics[width=0.11\textwidth,height=0.07\textwidth]{comp_iiw/zhou/118514-s.jpg} &         
%         \includegraphics[width=0.11\textwidth,height=0.07\textwidth]{comp_iiw/cg/118514-r.jpg}  & 
%         \includegraphics[width=0.11\textwidth,height=0.07\textwidth]{comp_iiw/cg/118514-s.jpg} &
%         \includegraphics[width=0.11\textwidth,height=0.07\textwidth]{comp_iiw/ffi/118514-albedo.png}& 
%         \includegraphics[width=0.11\textwidth,height=0.07\textwidth]{comp_iiw/ffi/118514-shading.png}

         \vspace{-1mm}
        \\                       
        {\scriptsize Image} & {\scriptsize Bell~\cite{bell2014intrinsic} ($A$)}  & {\scriptsize Bell~\cite{bell2014intrinsic}($S$)} & {\scriptsize Zhou~\cite{zhou2015learning} ($A$)}  & {\scriptsize Zhou \cite{zhou2015learning} ($S$)}  & {\scriptsize CGI \cite{cgintrinsic} ($A$)} & {\scriptsize CGI \cite{cgintrinsic} ($S$)}   &  {\scriptsize FFI-Net ($A$)} & {\scriptsize FFI-Net ($S$)}
    \end{tabular}  
  \caption{ Qualitative comparisons of (A)lebdo and (S)hading on IIW.
    % Our predictions show significant improvements compared to
    % state-of-the-art algorithms (bell~\etal ~\cite{bell2014intrinsic}
    % and zhou~\etal~\cite{zhou2015learning}). 
    % In particular, our
    % predicted shading channels include significantly less surface
    % texture in several challenging
    % settings.
    } \label{fig:iiw} 
\end{figure*}
\begin{figure}[htp]
\begin{center}
\resizebox{1.0\linewidth}{!}{
\begin{tabular}{c c ccccc}
\vspace{-0.5mm}
\!\!\includegraphics[width=1.4cm,height=1.cm]{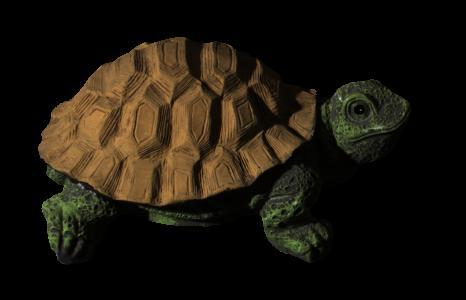}
& \raisebox{3mm}{\rotatebox{0}{(A)}}
&\includegraphics[width=1.4cm,height=1.cm]{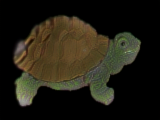}
&\includegraphics[width=1.4cm,height=1.cm]{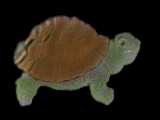}
&\includegraphics[width=1.4cm,height=1.cm]{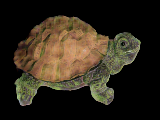}
&\includegraphics[width=1.4cm,height=1.cm]{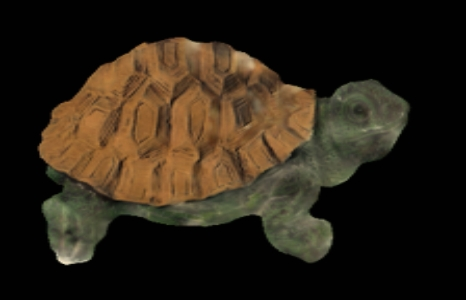}
&\includegraphics[width=1.4cm,,height=1cm]{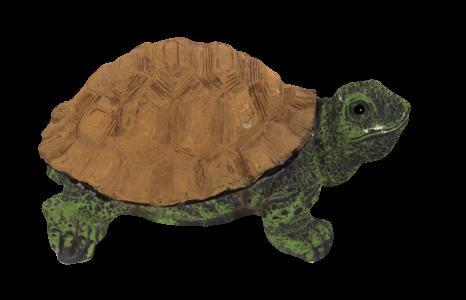}
\cr
& \raisebox{3mm}{\rotatebox{0}{(S)}}
&\includegraphics[width=1.4cm,height=1.cm]{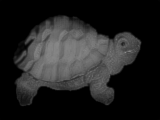}
&\includegraphics[width=1.4cm,height=1.cm]{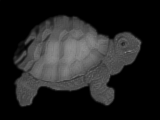}
&\includegraphics[width=1.4cm,height=1.cm]{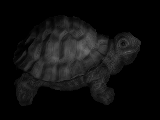}
&\includegraphics[width=1.4cm,height=1.cm]{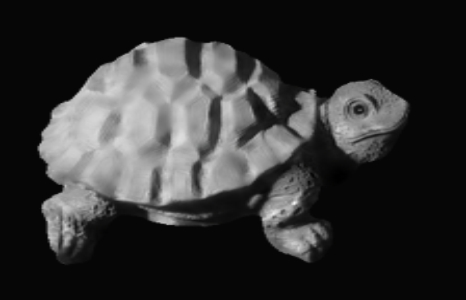}
&\includegraphics[width=1.4cm,height=1.cm]{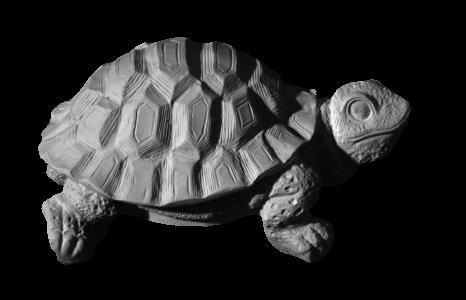}
\\

\vspace{-0.5mm}

\!\!\includegraphics[width=1.4cm]{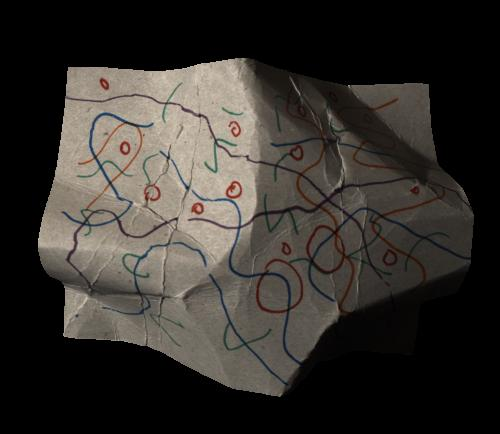}
& \raisebox{3mm}{\rotatebox{0}{(A)}}
&\includegraphics[width=1.4cm,height=1.215cm]{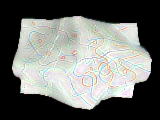}
&\includegraphics[width=1.4cm,height=1.215cm]{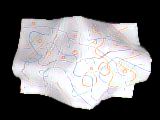}
&\includegraphics[width=1.4cm,height=1.215cm]{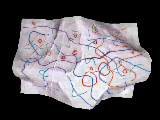}
&\includegraphics[width=1.4cm, height=1.215cm]{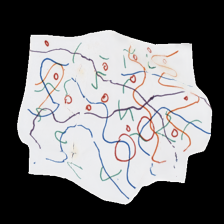}
&\includegraphics[width=1.4cm,height=1.215cm]{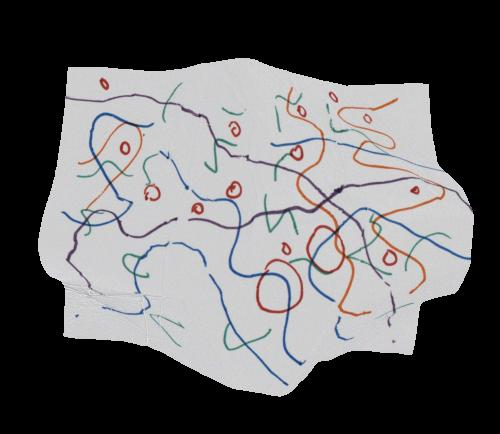}\\
& \raisebox{3mm}{\rotatebox{0}{(S)}}
&\includegraphics[width=1.4cm,height=1.215cm]{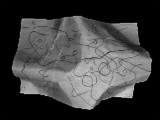}
&\includegraphics[width=1.4cm,height=1.215cm]{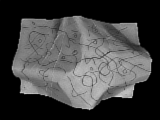}
&\includegraphics[width=1.4cm,height=1.215cm]{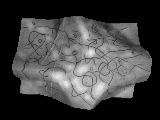}
&\includegraphics[width=1.4cm, height=1.215cm]{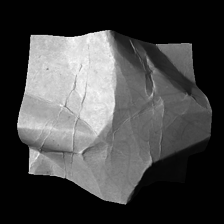}
&\includegraphics[width=1.4cm,height=1.215cm]{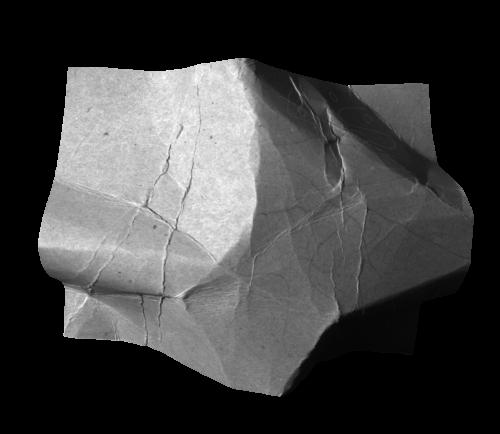}\\

\vspace{-0.5mm}

\small{Input} & & IntriNet  & IntriNet  & Retinet & \small{FFI-Net} & \small{Ground Truth}\\
 & & w/o imf\cite{baslamisli2018cnn} &  w/ imf\cite{baslamisli2018cnn} & \cite{baslamisli2018cnn} &  & \\

% \vspace{-0.6mm}

% &\multicolumn{4}{ c }{\small{Albedo}} & \multicolumn{4}{ c }{\small{Shading}}\\
\end{tabular}}

\end{center}
\vspace{-2mm}
\caption{Sample  (A)lbedo and (S)hading on MIT Intrinsic. Comparison with different versions in~\cite{baslamisli2018cnn}. Results of~\cite{baslamisli2018cnn} are downloaded from their project webpage.
%Only trained on MIT itself, our method can produce visually-pleasing output, similiar to Fan \textit{et al.} \cite{fan2018revisiting}
}
\vspace{-3mm}
\label{figure:mit2}
\end{figure}

\begin{figure}[t]
\begin{center}

\begin{tabular}{ccc}

\vspace{-0.75mm}
\raisebox{.9\height}{\rotatebox{90}{\scriptsize{{Input}}}}
&\multicolumn{2}{c}{\includegraphics[width=3.6cm]{comp-mpi-imagesplit/2-input.jpg}}
\\
& (A) & (S) \\
% \vspace{-0.75mm}
% \raisebox{0.5\height}{\rotatebox{90}{\scriptsize{{Lee~\cite{lee2012estimation}}}}}
% &{{\includegraphics[width=3.6cm]{comp-mpi-imagesplit/2-predict-albedo-lee.jpg}}}
% &{{\includegraphics[width=3.6cm]{comp-mpi-imagesplit/2-predict-shading-lee.jpg}}}
% \\

\vspace{-0.75mm}
\raisebox{0.5\height}{\rotatebox{90}{\scriptsize{{Barron~\cite{barron2015shape}}}}}
&{{\includegraphics[width=3.6cm]{comp-mpi-imagesplit/2-predict-albedo-barron.jpg}}}
&{{\includegraphics[width=3.6cm]{comp-mpi-imagesplit/2-predict-shading-barron.jpg}}}
\\

\vspace{-0.75mm}
\raisebox{0.5\height}{\rotatebox{90}{\scriptsize{{Chen~\cite{chen2013simple}}}}}
&{{\includegraphics[width=3.6cm]{comp-mpi-imagesplit/2-predict-albedo-chen.jpg}}}
&{{\includegraphics[width=3.6cm]{comp-mpi-imagesplit/2-predict-shading-chen.jpg}}}
\\

\vspace{-0.75mm}
\raisebox{1\height}{\rotatebox{90}{\scriptsize{{DI~\cite{narihira2015direct}}}}}
&{{\includegraphics[width=3.6cm]{comp-mpi-imagesplit/2-predict-albedo-di.jpg}}}
&{{\includegraphics[width=3.6cm]{comp-mpi-imagesplit/2-predict-shading-di.jpg}}}
\\

\vspace{-0.75mm}
\raisebox{1\height}{\rotatebox{90}{\scriptsize{{Fan \cite{fan2018revisiting}}}}}
&{{\includegraphics[width=3.6cm]{comp-mpi-imagesplit/2-predict-albedo-fan.jpg}}}
&{{\includegraphics[width=3.6cm]{comp-mpi-imagesplit/2-predict-shading-fan.jpg}}}
\\

\vspace{-0.75mm}
\raisebox{1\height}{\rotatebox{90}{\scriptsize{{Lap\cite{cheng2018intrinsic}}}}}
&{{\includegraphics[width=3.6cm]{comp-mpi-imagesplit/2-predict-albedo-lap.jpg}}}
&{{\includegraphics[width=3.6cm]{comp-mpi-imagesplit/2-predict-shading-lap.jpg}}}
\\

\vspace{-0.75mm}
\raisebox{1\height}{\rotatebox{90}{\scriptsize{{~~~~FFI}}}}
&{{\includegraphics[width=3.6cm]{comp-mpi-imagesplit/2-predict-albedo-fft.png}}}
&{{\includegraphics[width=3.6cm]{comp-mpi-imagesplit/2-predict-shading-fft.png}}}
\\

\vspace{-0.75mm}
{\rotatebox{90}{\scriptsize{{Ground Truth}}}}
&{{\includegraphics[width=3.6cm]{comp-mpi-imagesplit/2-label-albedo-mark.jpg}}}
&{{\includegraphics[width=3.6cm]{comp-mpi-imagesplit/2-label-shading-mark.jpg}}}
\\
\vspace{-5mm}

\end{tabular}

\end{center}
\vspace{-2.5mm}
\caption{More Examples of (A)lbedo and (S)hading predictions on MPI-Sintel (image split). %FFI-Net performs well in difficult parts, \eg hair bunchesa and  cast shadows.
}
\label{figure:mpi_imagesplit_supple}
\vspace{-3mm}
\end{figure}

%Compared to state-of-the-art method MSCR \cite{DI2015}, we show much sharper effects and better performance.

\section{More Examples for Visualization}
\begin{itemize}
    \item Fig. \ref{figure:mpi_scenesplit_supple} and Fig. \ref{figure:mpi_imagesplit_supple}: visual results on MPI-Sintel dataset with scene split and image split, respectively. We compare our method with~\cite{fan2018revisiting,narihira2015direct,chen2013simple,cheng2018intrinsic,barron2015shape}. We particularly point the readers to the flatten patches and fine textures (see red arrows) in the images to show the superiority of our method. 
   % \vspace{-2mm}
%    \item Fig. \ref{figure:mpi_imagesplit_supple}: visual results on MPI-Sintel imagesplit. 
    \vspace{-2mm}
    \item %Fig.~\ref{figure:mit-supple} and
    Fig.~\ref{figure:mit2}: more visual results on MIT Intrinsic dataset. In %Fig.～\ref{figure:mit-supple} we compare our method with~\cite{shi2017learning,narihira2015direct,fan2018revisiting}. While 
     Fig.~\ref{figure:mit2} we compare our FFI-Net with different versions in~\cite{baslamisli2018cnn}; ours are clearly visually better than~\cite{baslamisli2018cnn}. 
    \vspace{-2mm}
    \item Fig.~\ref{fig:iiw}: visual results on IIW benchmark. We compare our FFI-Net with other representative approaches~\cite{bell2014intrinsic,zhou2015learning,cgintrinsic}.
   % \vspace{-2mm}
%    \item Fig.~\ref{figure:mit2}: visual comparison with a state-of-the-art method~\cite{baslamisli2018cnn} on MIT Intrinsic.
\end{itemize}
